# Supplementary material for: Transferable Latent-to-Latent Locomotion Policy for Efficient and Versatile Motion Control of Diverse Legged Robots
Source: arXiv:2503.17626 source file (2025-03-22)
Supplement: Supplementary file 1 [file Appendix.tex]

\section{Appendix of Proofs}

\section{Appendix of Experiments}

\subsection{Implementation details}
\label{app:impd}

\subsubsection{Simulation implementation}

\subsubsection{Observation components}

We first examine our method with a simpler observation construction and also serve as the oracle policy, for the real world policy we use a much complex construction. 

Adapting a distillation strategy.
